# Supplementary material for: Artificial diffusion for convective and acoustic low Mach number flows I: Analysis of the modified equations, and application to Roe-type schemes
Source: arXiv:2112.08977 source file (2023-03-22)
Supplement: Supplementary file 1 [file asymptotic_notation.tex]

The standard definition of big-O ($\mathcal{O}$) is as an upper bound, i.e.
\[
    f(M)\sim\mathcalOM{n} \;\Rightarrow\; |f(M)|<(c_f M^n) \; \forall \; M<c_0
\]
where $c_f$ and $c_0$ are constants which do not depend on M.
For our application, $c_f$ and $c_0$ may rely on any flow condition or material property other than the Mach number, although $c_0$ will usually be somewhere around 0.2, where compressibility effects become small.

In section ** we are concerned with finding (and designing) limit equations, where only the largest terms remain as $M\to0$, for which a bound is an insufficient metric.
For example, both terms in $f(M) = M^3 + M^2$ are $\mathcalOM{2}$ as $M\to0$ under the definition above, however only $M^2$ remains in the limit equation.
If we use $M^2$ as analogous to the convection (l.h.s.) terms in a modified equation, and $M^3$ as analogous to the diffusion (r.h.s.) terms in a modified equation, then $f(M)$ has asymptotically vanishing diffusion, even though $(r.h.s)\sim\mathcal{O}(l.h.s.)$ as $M\to0$.

Instead, we will a use more restrictive definition:
\[
    f(M)\sim\mathcalOM{n} \;\Rightarrow\; |f(M)|\approx (c_f M^n) \; \forall \; M<c_0
\]
Or, more formally:
\[
    f(M) \sim \mathcalOM{n} \; \Rightarrow \; \exists \; c_f \in \mathbb{R}\; \textrm{s.t.}\; \forall \varepsilon>0 \;\exists\; \delta>0 \;\textrm{s.t.}\; | f(M) - c_f M^n |<\varepsilon \; \forall \: M<\delta
\]
Which can be read as: if $f(M)\sim\mathcalOM{n}$, then $f(M)$ can be made arbitrarily close to the function $c_f M^n$ for some constant $c_f$ by simply taking M small enough.

We will also (mis-)use the \textit{less-than-approximately} and \textit{greater-than-approximately} symbols to mean, respectively, \textit{asymptotically-less-than} or \textit{asymptotically-greater-than} in the limit as $M\to0$:
\begin{alignat*}{2}
    g(M) \lesssim \mathcalOM{n} \; & \Rightarrow \; g(M) \sim \mathcalOM{m}, \quad & m>n \\
    h(M) \gtrsim  \mathcalOM{n} \; & \Rightarrow \; h(M) \sim \mathcalOM{l}, \quad & l<n
\end{alignat*}
Lastly, where terms are independent of $M$ we use $\mathcalOM{0}$ instead of $\mathcal{O}(1)$, to be clear we do not mean that the order of magnitude is necessarily on the order of unity.
